# Supplementary material for: Accelerated Recovery with RIS: Designing Wireless Resilience in Mission-Critical Environments
Source: arXiv:2504.11589 source file (2026-04-27)
Supplement: Supplementary file 1 [file appendix.tex]

%%% remove blank page at beginning of appendix?
%% \makeatletter\@openrightfalse\makeatother
%%% to preamble
%
%\newcommand{\shatab}[2]{$K_{#1}$ & \texttt{#2} \\}
%
%\section{Appendix}\label{chap:appendix}
%
%\section*{SHA--512: Constants}
%\begin{table}[!h]
%\caption{Constants used during the calculation of a SHA--512 hash value.}\label{app:sha-const}
%\begin{minipage}{.45\textwidth}
%\centering
%\begin{tabular}{ll} \toprule \addlinespace
%Constant & Value (hexadecimal) \\ \addlinespace \midrule \addlinespace
%\shatab{0}{428a2f98d728ae22}
%\shatab{1}{7137449123ef65cd}
%\shatab{2}{b5c0fbcfec4d3b2f}
%\shatab{3}{e9b5dba58189dbbc}
%\shatab{4}{3956c25bf348b538}
%\shatab{5}{59f111f1b605d019}
%\shatab{6}{923f82a4af194f9b}
%\shatab{7}{ab1c5ed5da6d8118}
%\shatab{8}{d807aa98a3030242}
%\shatab{9}{12835b0145706fbe}
%\shatab{10}{243185be4ee4b28c}
%\shatab{11}{550c7dc3d5ffb4e2}
%\shatab{12}{72be5d74f27b896f}
%\shatab{13}{80deb1fe3b1696b1}
%\shatab{14}{9bdc06a725c71235}
%\shatab{15}{c19bf174cf692694}
%\shatab{16}{e49b69c19ef14ad2}
%\shatab{17}{efbe4786384f25e3}
%\shatab{18}{0fc19dc68b8cd5b5}
%\shatab{19}{240ca1cc77ac9c65}
%\shatab{20}{2de92c6f592b0275}
%\shatab{21}{4a7484aa6ea6e483}
%\shatab{22}{5cb0a9dcbd41fbd4}
%\shatab{23}{76f988da831153b5}
%\shatab{24}{983e5152ee66dfab}
%\shatab{25}{a831c66d2db43210}
%\shatab{26}{b00327c898fb213f}
%\shatab{27}{bf597fc7beef0ee4}
%\shatab{28}{c6e00bf33da88fc2}
%\shatab{29}{d5a79147930aa725}
%\end{tabular}
%\end{minipage}
%\hfill
%\begin{minipage}{.45\textwidth}
%\centering
%\begin{tabular}{ll} \toprule \addlinespace
%Constant & Value (hexadecimal) \\ \addlinespace \midrule \addlinespace
%\shatab{30}{06ca6351e003826f}
%\shatab{31}{142929670a0e6e70}
%\shatab{32}{27b70a8546d22ffc}
%\shatab{33}{2e1b21385c26c926}
%\shatab{34}{4d2c6dfc5ac42aed}
%\shatab{35}{53380d139d95b3df}
%\shatab{36}{650a73548baf63de}
%\shatab{37}{766a0abb3c77b2a8}
%\shatab{38}{81c2c92e47edaee6}
%\shatab{39}{92722c851482353b}
%\shatab{40}{a2bfe8a14cf10364}
%\shatab{41}{a81a664bbc423001}
%\shatab{42}{c24b8b70d0f89791}
%\shatab{43}{c76c51a30654be30}
%\shatab{44}{d192e819d6ef5218}
%\shatab{45}{d69906245565a910}
%\shatab{46}{f40e35855771202a}
%\shatab{47}{106aa07032bbd1b8}
%\shatab{48}{19a4c116b8d2d0c8}
%\shatab{49}{1e376c085141ab53}
%\shatab{50}{2748774cdf8eeb99}
%\shatab{51}{34b0bcb5e19b48a8}
%\shatab{52}{391c0cb3c5c95a63}
%\shatab{53}{4ed8aa4ae3418acb}
%\shatab{54}{5b9cca4f7763e373}
%\shatab{55}{682e6ff3d6b2b8a3}
%\shatab{56}{748f82ee5defb2fc}
%\shatab{57}{78a5636f43172f60}
%\shatab{58}{84c87814a1f0ab72}
%\shatab{59}{8cc702081a6439ec}
%\end{tabular}
%\end{minipage}
%\end{table}
%
%\clearpage
%
%\begin{table}[!h]
%\caption{Constants used during the calculation of a SHA--512 hash value. (Cont.)}\label{app:sha-const2}
%\begin{minipage}{.45\textwidth}
%\centering
%\begin{tabular}{ll} \toprule \addlinespace
%Constant & Value (hexadecimal) \\ \addlinespace \midrule \addlinespace
%\shatab{60}{90befffa23631e28}
%\shatab{61}{a4506cebde82bde9}
%\shatab{62}{bef9a3f7b2c67915}
%\shatab{63}{c67178f2e372532b}
%\shatab{64}{ca273eceea26619c}
%\shatab{65}{d186b8c721c0c207}
%\shatab{66}{eada7dd6cde0eb1e}
%\shatab{67}{f57d4f7fee6ed178}
%\shatab{68}{06f067aa72176fba}
%\shatab{69}{0a637dc5a2c898a6}
%\addlinespace\bottomrule
%\end{tabular}
%\end{minipage}
%\hfill
%\begin{minipage}{.45\textwidth}
%\centering
%\begin{tabular}{ll} \toprule \addlinespace
%Constant & Value (hexadecimal) \\ \addlinespace \midrule \addlinespace
%\shatab{70}{113f9804bef90dae}
%\shatab{71}{1b710b35131c471b}
%\shatab{72}{28db77f523047d84}
%\shatab{73}{32caab7b40c72493}
%\shatab{74}{3c9ebe0a15c9bebc}
%\shatab{75}{431d67c49c100d4c}
%\shatab{76}{4cc5d4becb3e42b6}
%\shatab{77}{597f299cfc657e2a}
%\shatab{78}{5fcb6fab3ad6faec}
%\shatab{79}{6c44198c4a475817}
%\addlinespace\bottomrule
%\end{tabular}
%\end{minipage}
%\end{table}
%
%\section*{SHA--512: Initial Hash $H^{(0)}$}
%\begin{table}[!h]
%\centering
%\caption{Initial hash value for SHA--512.}\label{app:sha-init}
%\begin{tabular}{ll} \toprule \addlinespace
%$H_i^{(0)}$ & Value (hexadecimal) \\ \addlinespace \midrule \addlinespace
%$H_0^{(0)}$ & \texttt{6a09e667f3bcc908} \\
%$H_1^{(0)}$ & \texttt{bb67ae8584caa73b} \\
%$H_2^{(0)}$ & \texttt{3c6ef372fe94f82b} \\
%$H_3^{(0)}$ & \texttt{a54ff53a5f1d36f1} \\
%$H_4^{(0)}$ & \texttt{510e527fade682d1} \\
%$H_5^{(0)}$ & \texttt{9b05688c2b3e6c1f} \\
%$H_6^{(0)}$ & \texttt{1f83d9abfb41bd6b} \\
%$H_7^{(0)}$ & \texttt{5be0cd19137e2179} \\
%\addlinespace\bottomrule
%\end{tabular}
%\end{table}
%
%
%\section*{SHA--512: Algorithm}
%Algorithm~\ref{alg:sha512} shows the complete algorithm for calculating the hash digest of a message that is split into $M^{(1)},\dots,M^{(N)}$ blocks according to Section~\ref{subsec:sha}.
%%\begin{algorithm}[!h]                      % enter the algorithm environment
%%\caption{\textsc{SHA--512}}          % give the algorithm a caption
%%\label{alg:sha512}                           % and a label for \ref{} commands later in the document
%\begin{center}
%\captionsetup{style=ruled,type=algorithm,skip=0pt}
%\makeatletter
%\fst@algorithm\@fs@pre
%\makeatother
%\caption{\textsc{SHA--512}}          % give the algorithm a caption
%\makeatletter
%\@fs@mid\vspace{2pt}
%\makeatother
%\label{alg:sha512}
%\begin{algorithmic}[1]                    % enter the algorithmic environment
%\REQUIRE Message blocks $M^{(1)}$ to $M^{(N)} \in \mathcal{M}$
%\ENSURE SHA--512 hash value $H$ of $\mathcal{M}$
%	\FOR{$i = 1$ to $N$}
%		\STATE Prepare message schedule $W_t$:
%			\begin{align*}
%			W_t = \left\{\begin{array}{cr}
%			M_t^{(i)}, & 0 \le t \le 15 \\
%			\sigma_1\left(W_{t-2}\right)+W_{t-7}+\sigma_0\left(W_{t-15}\right)+W_{t-16}, & 16 \le t \le 79
%			\end{array}\right.
%			\end{align*}
%		\STATE Initialize working variables $a, b, c, d, e, f, g, h$ with $(i-1)^{\text{st}}$ hash value:
%			\begin{align*}
%			a & = H_0^{(i-1)} \\
%			b & = H_1^{(i-1)} \\
%			c & = H_2^{(i-1)} \\
%			d & = H_3^{(i-1)} \\
%			e & = H_4^{(i-1)} \\
%			f & = H_5^{(i-1)} \\
%			g & = H_6^{(i-1)} \\
%			h & = H_7^{(i-1)}
%			\end{align*}
%		\FOR{$t = 0$ to $79$}
%			\STATE Calculate, whereas $T_1, T_2$ are temporary words:
%				\begin{align*}
%				T_1 &= h+\Sigma_1 (e) + \chi(e,f,g)+K_t+W_t, \\
%				T_2 &= \Sigma_0(a)+\Upsilon(a,b,c) \\
%				h &= g \\
%				g &= f \\
%				f &= e \\
%				e &= d+T_1 \\
%				d &= c \\
%				c &= b \\
%				b &= a \\
%				a &= T_1+T_2
%				\end{align*}
%		\ENDFOR
%		\STATE Compute the $i^{\,\text{th}}$ \emph{intermediate} hash value $H^{(i)}$:
%			\begin{align*}
%			H_0^{(i)} &= a+H_0^{(i-1)} \\
%			H_1^{(i)} &= b+H_1^{(i-1)} \\
%			H_2^{(i)} &= c+H_2^{(i-1)} \\
%			H_3^{(i)} &= d+H_3^{(i-1)} \\
%			H_4^{(i)} &= e+H_4^{(i-1)} \\
%			H_5^{(i)} &= f+H_5^{(i-1)} \\
%			H_6^{(i)} &= g+H_6^{(i-1)} \\
%			H_7^{(i)} &= h+H_7^{(i-1)} \\
%			\end{align*}
%	\ENDFOR
%	\STATE Concatenate the intermediate hash values of the $N^{\text{th}}$ round to the output hash:
%	\begin{align*}
%	H \leftarrow H_0^{(N)} \left\| H_1^{(N)} \left\| H_2^{(N)} \left\| H_3^{(N)} \left\| H_4^{(N)} \left\| H_5^{(N)} \left\| H_6^{(N)} \left\| H_7^{(N)}\right.\right.\right.\right.\right.\right.\right.
%	\end{align*}
%\end{algorithmic}
%\makeatletter
%\vspace{2pt}\@fs@post
%\makeatother
%\end{center}
